# Supplementary material for: Behind the Intent of Extract Method Refactoring: A Systematic Literature Review
Source: arXiv:2312.12600 source file (2023-12-19)
Supplement: Supplementary file 2 [file 09-appendix.tex]

\section{Appendix}
\label{Section:Appendix}

\begin{table}
  \centering
	 \caption{\textit{Extract Method} refactoring tools.}
	 \label{Table:Tool_Characteristics}
  %\vspace{0.5cm}

%\begin{adjustbox}{width=1.05\textwidth,center}
\rowcolors{2}{white}{gray!25}
\begin{tabular}{lllllllllll}\hline
\toprule
\bfseries Tool & \bfseries Tool Link & \bfseries Last Update \\
\midrule

  \textbf{Tuck} \cite{lakhotia1998restructuring} &    Unknown &   Unknown\\
\textcolor{black}{\textbf{CloRT}} \cite{balazinska1999partial} & \textcolor{black}{Unknown} & \textcolor{black}{Unknown} \\
\textcolor{black}{\textbf{Nate}} \cite{ettinger2004untangling} & \textcolor{black}{Unknown} & \textcolor{black}{Unknown} \\

   \textbf{CCShaper} \cite{higo2004refactoring} &      Unknown &     Unknown \\

   \textbf{Aries} \cite{higo2004aries,higo2005aries,higo2008metric}  &    Unknown &     Unknown \\ 

  \textbf{SDAR} \cite{o2005star}  &   Unknown&    Unknown \\ %\hline 

   \textbf{Xrefactory} \cite{vittek2007c++}  &    \cite{Xrefactory} &    2007 \\ %\hline

%\hline

  \textbf{Unnamed} \cite{corbat2007ruby}  &   \cite{Unnamed3} &   2012 \\ %\hline 

   \textbf{RefactoringAnnotation} \cite{murphy2008breaking} &       Unknown &     Unknown \\ %\hline

  \textbf{JDeodorant}~\cite{tsantalis2009identification,tsantalis2011identification,krishnan2013refactoring,krishnan2014unification,tsantalis2015assessing,mazinanian2016jdeodorant,tsantalis2017clone} &      \cite{Jdeodorant} &   2019 \\

   \multirow{1}{*}{\textbf{AutoMed}~\cite{yang2009identifying}}  &   Unknown &     Unknown\\ %\hline

   \multirow{1}{*}{\textbf{Wrangler}~\cite{li2009clone}}  &   \cite{Wrangler} &     2023\\ %\hline

   \multirow{1}{*}{\textbf{HaRe}~\cite{brown2010clone}}  &   \cite{HaRe} &     2017\\ %\hline

  \multirow{1}{*} {\textbf{ReAF}~\cite{kanemitsu2011visualization}} &    Unknown &   Unknown  \\ %\hline

   \textbf{Unnamed} \cite{cousot2012abstract}  &    Unknown&     Unknown \\ %\hline

  \textbf{CeDAR} \cite{tairas2012increasing} &   Unknown &   Unknown  \\ %\hline

\textcolor{black}{\textbf{FTMPAT} \cite{goto2013extract}} & \textcolor{black}{Unknown} & \textcolor{black}{Unknown}  \\

   \textbf{SPAPE} \cite{bian2013spape} &   Unknown &     Unknown \\ %\hline

  \textbf{JExtract}~\cite{silva2014recommending,silva2015jextract}  &   \cite{JExtract} &   2016 \\

   \multirow{1}{*} {\textbf{DCRA} \cite{arcelli2015duplicated}}  &    Unknown&     Unknown \\ %\hline

\textcolor{black}{\textbf{RASE}} \cite{meng2015does} & \cite{RASE} & \textcolor{black}{2015} \\

  \textbf{SEMI}~\cite{charalampidou2016identifying} &   \cite{SEMI}&   2016\\

%\textbf{ConQAT}~\cite{haas2016deriving,haas2017learning} & Java   & 1  & Unknown & Yes & \cite{ConQAT} & 2015\\ %\hline

  \textbf{GEMS}~\cite{xu2017gems}  &   \cite{GEMS} &   2017\\ 

   \textbf{PostponableRefactoring} \cite{maruyama2017tool} &      \cite{PostponableRefactoring} &    2018 \\ %\hline

  \textbf{LLPM} \cite{xu2017log} &   Unknown &   Unknown \\

\textcolor{black}{\textbf{PRI}} \cite{chen2017tool} &  \textcolor{black}{Unknown} & \textcolor{black}{Unknown} \\

   \textbf{LMR} \cite{meananeatra2018refactoring} &       Unknown &     Unknown \\ %\hline

  \multirow{1}{*}{\textbf{CREC}~\cite{yue2018automatic}} &     \cite{CREC} &   2018 \\ %\hline

\textcolor{black}{\textbf{Bandago}} \cite{vidal2018assessing} &  \textcolor{black}{Unknown}& \textcolor{black}{Unknown}\\

\textcolor{black}{\textbf{Unnamed}} \cite{shin2019study} & \textcolor{black}{Unknown}& \textcolor{black}{Unknown}\\

   \multirow{1}{*} {\textbf{Unnamed}~\cite{yoshida2019proactive}} &    \cite{Unnamed2} &    2019 \\ %\hline

    \multirow{1}{*} {\textbf{CloneRefactor}~\cite{baars2019towards}} &   \cite{CloneRefactor} &    2020 \\ %\hline

  \multirow{1}{*} {\textbf{\textcolor{black}{TOAD}} \cite{antezana2019toad,alcocer2020improving}} &   \cite{TOAD} &   2019\\ %\hline
%Unnamed \cite{abid2020does} & Java & No specific context & & & N/A & Yes &  \\ \hline
\textbf{Segmentation}~\cite{tiwari2022identifying} & \cite{Segmentation} & 2022 \\

  \multirow{1}{*}{\textbf{LiveRef} \cite{fernandes2022liveref,fernandes2022live}} &    \cite{LiveRef} &   2022 \\ %\hline
  
\textbf{AntiCopyPaster} \cite{alomar2022anticopypaster,alomar2023just}  & \cite{AntiCopyPaster} &  2023 \\

\textcolor{black}{\textbf{REM} \cite{thy15adventure}} &  \textcolor{black}{\cite{REM}} & \textcolor{black}{2023}  \\

\bottomrule
\end{tabular}
%\end{adjustbox}

\vspace{-.3cm}
\end{table}
